# Supplementary material for: Compositional Image Decomposition with Diffusion Models
Source: arXiv:2406.19298 source file (2024-06-27)
Supplement: Supplementary file 1 [file supplemental.tex]

\documentclass{article}

\PassOptionsToPackage{numbers, compress}{natbib}
\usepackage{neurips_2023}

\input{packages}
\input{math_commands}
\input{defs}
\usepackage{Definitions}
\usepackage{wrapfig}
\usepackage[pagebackref=true,breaklinks=true,colorlinks,citecolor=gray]{hyperref}

\title{Unsupervised Compositional Image Decomposition with Diffusion Models Supplementary Material}

\author{%
  David S.~Hippocampus\thanks{Use footnote for providing further information
    about author (webpage, alternative address)---\emph{not} for acknowledging
    funding agencies.} \\
  Department of Computer Science\\
  Cranberry-Lemon University\\
  Pittsburgh, PA 15213 \\
  \texttt{hippo@cs.cranberry-lemon.edu} \\
}

\begin{document}

\maketitle
\appendix

\input{appendix}

{\small
\bibliographystyle{plainnat}
\bibliography{reference,neurips_2023}
}

\end{document}
